# Supplementary material for: Extracting Information from Stochastic Trajectories of Gene Expression
Source: arXiv:2206.14874 source file (2022-06-29)
Supplement: Supplementary file 1 [file supp.pdf]

# *Supplementary information for:* Extracting Information from Stochastic Trajectories of Gene Expression

Zachary R Fox

*Center for Nonlinear Studies (T-CNLS), Theoretical Division, Los Alamos National Laboratory, Los Alamos NM 87545 and Information Sciences Group (CCS-3), Computer, Computational and Statistical Sciences Division, Los Alamos National Laboratory, Los Alamos NM 87545*

(Dated: June 28, 2022)

## CONTENTS

S1. Chemical Master Equation and Finite State Projection S2

S2. Sensitivity analysis for Markov Jump Processes S3

S3. Derivation of Fisher information for Markovian Trajectories S4

S4. Comparing time-series and snapshot data S7

S5. Continuous time birth-death process S7

S6. Two-state gene expression model S8

S7. Relating Fisher information and Channel Capacity S10

A simple regulated gene S14

References S16

## S1. CHEMICAL MASTER EQUATION AND FINITE STATE PROJECTION

Trajectories of many physical systems can be described by continuous time Markov chains CTMCs [1]. Here, we consider the process of stochastic gene expression, the process by which cells create RNA and protein, which is typically referred to as the chemical master equation (CME) [2, 3]. Each state in the discrete state Markov process is defined $\mathbf{x}_i = [\zeta_1, \zeta_2, \ldots, \zeta_N]_i \in \mathbf{X} \subset \mathbb{Z}^N_{\geq 0}$. Transitions from state $\mathbf{x}_i + \psi_\nu$ to $\mathbf{x}_i$ occur in the infinitesimal time $dt$ with probability $w_\nu dt$. These transitions can be written into a (potentially) infinite matrix $\mathbf{A}$, which is often referred to as the infinitesimal generator of the process. The matrix $\mathbf{A}$ is typically used in the chemical master equation framework and can be approximated using the finite state projection (FSP) approach [4], in which the full matrix $\mathbf{A}$ is truncated, and one solves the finite set of ordinary differential equations $\frac{d}{dt}\mathbf{p} = \mathbf{A}\mathbf{p}$, where the probability vector $\mathbf{p}(t)$ describes the probability of each state $\mathbf{x}_i$ at time $t$.

In this work, we are interested paths, or trajectories, sampled at a subset of times $\mathcal{T} = [t_1, t_2, \ldots t_N]$. However, for most practical applications, measurements are made at regular intervals of $\Delta t$, often corresponding to the frame rate of the camera taking measurements. From the modeling perspective, this corresponds to finding the matrix of transition probabilities for the CTMC above that describes stochastic gene expression. Let us denote the probability of a transition from $\mathbf{x}_i$ to $\mathbf{x}_j$ in the matrix $\mathbf{P}_{ji}$. The time evolution of the process is then governed by the infinite set of ODEs

$$\frac{d}{dt}\mathbf{P} = \mathbf{A}(t, \theta)\mathbf{P}, \tag{S1}$$

where $\mathbf{A}$ is the generator matrix for the chemical master equation as described above, $\theta$ denotes the kinetic parameters of the system. While $\mathbf{A}$ could in general be a function of time, in this work we focus on autonomous systems in which $\mathbf{A}$ is a static object. The initial condition for the MJP in Eq. S1, $\mathbf{P}_0$ is the identity matrix $\mathbf{I}$ of the same dimension as $\mathbf{A}$. Analagous to the FSP formulation [4], we can define a set of states indexed by $\mathcal{J}$ which are of interest and require any reaction which leaves this finite state space to go to a sink state $g(t)$. Transitions into $g(t)$ are given by the sum of all jumps out of the state space

$$\frac{d}{dt}\begin{bmatrix}\mathbf{P}_{\mathcal{J}\mathcal{J}} & \mathbf{P}_{\mathcal{J}\mathcal{J}'} \\ \mathbf{P}_{\mathcal{J}'\mathcal{J}} & \mathbf{P}_{\mathcal{J}'\mathcal{J}'}\end{bmatrix} = \begin{bmatrix}\mathbf{A}_{\mathcal{J}\mathcal{J}} & \mathbf{A}_{\mathcal{J}\mathcal{J}'} \\ \mathbf{A}_{\mathcal{J}'\mathcal{J}} & \mathbf{A}_{\mathcal{J}'\mathcal{J}'}\end{bmatrix}\begin{bmatrix}\mathbf{P}_{\mathcal{J}\mathcal{J}} & \mathbf{P}_{\mathcal{J}\mathcal{J}'} \\ \mathbf{P}_{\mathcal{J}'\mathcal{J}} & \mathbf{P}_{\mathcal{J}'\mathcal{J}'}\end{bmatrix} \tag{S2}$$

which then becomes

$$\frac{d}{dt}\begin{bmatrix}\mathbf{P}^{\text{FSP}}_{\mathcal{J}\mathcal{J}} & \mathbf{0}\\ \mathbf{g} & \mathbf{0}\end{bmatrix} = \begin{bmatrix}\mathbf{A}_{\mathcal{J}\mathcal{J}} & \mathbf{0}\\ -\mathbb{1}^{\text{T}}\mathbf{A}_{\mathcal{J}\mathcal{J}} & \mathbf{0}\end{bmatrix}\begin{bmatrix}\mathbf{P}^{\text{FSP}}_{\mathcal{J}\mathcal{J}} & \mathbf{0}\\ \mathbf{g} & \mathbf{0}\end{bmatrix}. \tag{S3}$$

Once the the finite transition probability matrix $\mathbf{P}(\Delta t)$ has been computed, assuming trajectories are sampled every $\Delta t$ times, one can find a solution of the probabilities over the states at $n\Delta t$, $\mathbf{p}(n\Delta t) = (\mathbf{P}(\Delta t)^n)\mathbf{p}_0$.

## S2. SENSITIVITY ANALYSIS FOR MARKOV JUMP PROCESSES

Here, we derive a forward sensitivity analysis for the FSP-based Markov jump process described in Eq. S3, where we have simplified the notation for $\mathbf{A}_{\mathcal{J}\mathcal{J}} \equiv \mathbf{A}$ such that $\mathbf{A}$ denotes the finite rate matrix and $\mathbf{P}$ denotes the finite matrix of jump probabilities. The solution to these ODEs is given in integral form

$$\mathbf{P} = \mathbf{P}_0 + \int_t^{t+\tau} \mathbf{A}(s,\theta)\mathbf{P}ds. \tag{S4}$$

Taking the partial derivative with respect to a single parameter $\theta$, we have

$$\frac{\partial}{\partial\theta}\mathbf{P} = \frac{\partial}{\partial\theta}\mathbf{P}_0 + \frac{\partial}{\partial\theta}\int_t^{t+\tau} ds\mathbf{A}(s,\theta)\mathbf{P} \tag{S5}$$

$$= \frac{\partial}{\partial\theta}\mathbf{P}_0 + \int_t^{t+\tau} ds\frac{\partial}{\partial\theta}\mathbf{A}(s,\theta)\mathbf{P} + \mathbf{A}(s,\theta)\frac{\partial}{\partial\theta}\mathbf{P}. \tag{S6}$$

Taking the time derivative yields the joint set of ODEs of the transition probabilities $\mathbf{P}$ and the sensitivities $\mathbf{S}$,

$$\frac{d}{dt}\begin{bmatrix}\mathbf{P}\\ \mathbf{S}^{\theta}\end{bmatrix} = \underbrace{\begin{bmatrix}\mathbf{A} & \mathbf{0}\\ \mathbf{A}^{\theta} & \mathbf{A}\end{bmatrix}}_{\mathbf{M}}\underbrace{\begin{bmatrix}\mathbf{P}\\ \mathbf{S}^{\theta}\end{bmatrix}}_{\mathbf{\Psi}}, \tag{S7}$$

where $\mathbf{A}^{\theta} = \frac{\partial}{\partial\theta}\mathbf{A}$. Each entry of the matrix $\mathbf{S}^{\theta}_{ji}$ is the sensitivity of each transition probability to the parameter $\theta$. For convenience, we define a matrix $\mathbf{M}$ which is the combined generator and vector $\mathbf{\Psi}$ which is the combined vector, and therefore the set of ODEs in Eq. S7 is given by

$$\frac{d}{dt}\mathbf{\Psi} = \mathbf{M}\mathbf{\Psi} \tag{S8}$$

This set of ODEs is independent for each parameter, and therefore the sensitivities to each parameter can be computed in parallel across multiple processors. This forward sensitivity approach amounts to solving a set of ODEs which is twice the size of the MJP described in Eq. S3, and therefore generally is tractable for problems for which the MJP is also tractable.

## S3. DERIVATION OF FISHER INFORMATION FOR MARKOVIAN TRAJECTORIES

Now, we derive the Fisher information for sample paths of the CTMC. Let us define a trajectory sampled at regular intervals of $\Delta t$ $\vec{X}_t = [x(0), x(\Delta t), ..., x(N_t \Delta t)]$. The probability of this path is

$$\begin{aligned} P(\vec{X}_t) &= p(x(0), x(\Delta t), ..., x(N_t \Delta t) \\ &= p(x_0) \prod_{k=1}^{N_t} p(x_k | x_{k-1}) \end{aligned} \tag{S9}$$

and the log-probability is

$$\log P(\vec{X}_t) = \log p(x_0) + \sum_{k=1}^{N_t} \log p(x_k | x_{k-1}). \tag{S10}$$

The Fisher information is defined as the expectation of the derivative of the log-likelihood with respect to model parameter $\theta_i$ times the derivative of the log-likelihood with respect to $\theta_j$,

$$\mathcal{I}_{i,j} = \mathbb{E}\left[ \frac{\partial \log P(\vec{X}_t)}{\partial \theta_i} \frac{\partial \log P(\vec{X}_t)}{\partial \theta_j} \right], \tag{S11}$$

where the expectation is taken over the paths, $P(\vec{X}_t)$ [5, 6]. Let us simplify notation for partial derivatives and logarithms by defining $\ell(x) \triangleq \log p(x)$ and $\partial_i \triangleq \frac{\partial}{\partial \theta_i}$. Applying Eq. S10 to S11, we have

$$\begin{aligned} \mathcal{I}_{i,j} = \mathbb{E}\Big[ &\partial_i \ell(x_0) \partial_j \ell(x_0) \\ &+ \partial_i \ell(x_0) \sum_{k=1}^{N_t} \partial_j \ell(x_k | x_{k-1}) + \partial_j \ell(x_0) \sum_{k=1}^{N_t} \partial_i \ell(x_k | x_{k-1}) \\ &+ \sum_{k=1}^{N_t} \sum_{k'=1}^{N_t} \partial_i \ell(x_k | x_{k-1}) \partial_j \ell(x_{k'} | x_{k'-1}) \Big]. \end{aligned} \tag{S12}$$

Splitting the expectation, we have

$$\begin{aligned}\mathcal{I}_{i,j} &= \mathbb{E}\Big[\partial_i \ell(x_0)\partial_j \ell(x_0)\Big] \\ &+ \sum_{k=1}^{N_t} \mathbb{E}\Big[\partial_i \ell(x_0)\partial_j \ell(x_k|x_{k-1})\Big] + \sum_{k=1}^{N_t} \mathbb{E}\Big[\partial_j \ell(x_0)\partial_i \ell(x_k|x_{k-1})\Big] \\ &+ \sum_{k=1}^{N_t}\sum_{k'=1}^{N_t} \mathbb{E}\Big[\partial_i \ell(x_k|x_{k-1})\partial_j \ell(x_{k'}|x_{k'-1})\Big].\end{aligned} \tag{S13}$$

The first expectation is the information in the initial distribution. The middle expectations are zero [6]:

$$\sum_{k=1}^{N_t} \mathbb{E}\Big[\partial_i \ell(x_0)\partial_j \ell(x_k|x_{k-1})\Big] = \sum_{k=1}^{N_t} \int D\vec{X}_t \partial_i \ell(x_0)\partial_j \ell(x_k|x_{k-1}) P(\vec{X}_t) = 0 \tag{S14}$$

$$\tag{S15}$$

The third expectation is the information in the transition probabilities:

$$= \sum_{k,k'=1}^{N_t} \int D\vec{X}_t \partial_i \ell(x_k|x_{k-1})\partial_j \ell(x_{k'}|x_{k'-1}) P(\vec{X}_t). \tag{S16}$$

Expanding this third expectation, if $k \neq k'$ the expectation is zero, so we are left with

$$= \sum_{k=1}^{N_t} \int D\vec{X}_t \partial_i \ell(x_k|x_{k-1})\partial_j \ell(x_k|x_{k-1}) P(\vec{X}_t). \tag{S17}$$

$$= \sum_{k=1}^{N_t} \int dx_0 dx_1 dx_2 \dots dx_{N_t} \partial_i \ell(x_k|x_{k-1})\partial_j \ell(x_k|x_{k-1}) p(x_0) \prod_{k'=1}^{N_t} p(x_{k'}|x_{k'-1}) \tag{S18}$$

Because we are considering finite state CTMCs, the path integral in the above equations can be rewritten as sums over the finite state space. Consider a single variable $x \in \mathbb{Z} \in [0, N]$, and a trajectory with only three measurements, $N_t = 3$, and two parameters $\theta = [\alpha, \beta]$. From the discrete path integral formulation above, the expectation from Eq. S18 has the following sums:

$$\begin{aligned}&= \sum_{j=1}^{N}\sum_{k=1}^{N}\sum_{l=1}^{N}\sum_{m=1}^{N} \Big[\partial_\beta p(x_1^{(k)}|x_0^{(j)})\partial_\alpha p(x_1^{(k)}|x_0^{(j)})\Big] \frac{p(x_0^{(j)})p(x_2^{(l)}|x_1^{(k)})p(x_3^{(m)}|x_2^{(l)})}{p(x_1^{(k)}|x_0^{(j)})} \\ &+ \sum_{j=1}^{N}\sum_{k=1}^{N}\sum_{l=1}^{N}\sum_{m=1}^{N} \Big[\partial_\beta p(x_2^{(l)}|x_1^{(k)})\partial_\alpha p(x_2^{(l)}|x_1^{(k)})\Big] \frac{p(x_0^{(j)})p(x_1^{(k)}|x_0^{(j)})p(x_3^{(m)}|x_2^{(l)})}{p(x_2^{(l)}|x_1^{(k)})} \\ &+ \sum_{j=1}^{N}\sum_{k=1}^{N}\sum_{l=1}^{N}\sum_{m=1}^{N} \Big[\partial_\beta p(x_3^{(m)}|x_2^{(l)})\partial_\alpha p(x_3^{(m)}|x_2^{(l)})\Big] \frac{p(x_0^{(j)})p(x_2^{(l)}|x_1^{(k)})p(x_1^{(k)}|x_0^{(j)})}{p(x_3^{(m)}|x_2^{(l)})}.\end{aligned} \tag{S19}$$

These sums can be written as simple matrix multiplications using the transition probabilities $\mathbf{P}$ found using Eq. S7, i.e. $\mathbf{P}_{ij} = p(x^{(i)}|x^{(j)})$ and the sensitivities $\mathbf{S}^{\alpha}_{ij} = \partial_\alpha p(x^{(i)}|x^{(j)})$. Finally, we define a matrix $\mathbf{Z}$ such that $\mathbf{Z}^{(\alpha\beta)}_{ij} = \frac{\mathbf{S}^{\alpha}_{ij}\mathbf{S}^{\beta}_{ij}}{\mathbf{P}_{ij}}$. With these definitions in hand, the sums in Eq. S19 can be written:

$$= \mathbb{1}^{\mathrm{T}}(\mathbf{P}\mathbf{P}\mathbf{Z}^{(\alpha\beta)}\mathbf{p}_0) + \mathbb{1}^{\mathrm{T}}(\mathbf{P}\mathbf{Z}^{(\alpha\beta)}\mathbf{P}\mathbf{p}_0) + \mathbb{1}^{\mathrm{T}}(\mathbf{Z}^{(\alpha\beta)}\mathbf{P}\mathbf{P}\mathbf{p}_0) \tag{S20}$$

$$= \mathbb{1}^{\mathrm{T}}((\mathbf{P}\mathbf{P}\mathbf{Z}^{(\alpha\beta)}\mathbf{p}_0 + \mathbf{P}\mathbf{Z}^{(\alpha\beta)}\mathbf{P}\mathbf{p}_0 + \mathbf{Z}^{(\alpha\beta)}\mathbf{P}\mathbf{P}\mathbf{p}_0) \tag{S21}$$

$$= \mathbb{1}^{\mathrm{T}}(\mathbf{P}\mathbf{P}\mathbf{Z}^{(\alpha\beta)} + \mathbf{P}\mathbf{Z}^{(\alpha\beta)}\mathbf{P} + \mathbf{Z}^{(\alpha\beta)}\mathbf{P}\mathbf{P})\mathbf{p}_0. \tag{S22}$$

In general, we can write this for trajectories of length $N_t$ as

$$= \mathbb{1}^{\mathrm{T}}\left(\sum_{k=0}^{N_t-1} \mathbf{P}^{N_t-k}\mathbf{Z}^{(\alpha\beta)}\mathbf{P}^{k}\right)\mathbf{p}_0. \tag{S23}$$

Note that because $\mathbf{P}^k$ is Markovian, and therefore $\mathbb{1}^{\mathrm{T}}\mathbf{P}^k$ is equal to $\mathbb{1}^{\mathrm{T}}$. Including Eq. S23 and the information in the initial distribution, we have the total CTMC based Fisher information for trajectories to be

$$\mathcal{I}^{ts} = \underbrace{\mathbb{1}^{\mathrm{T}}\left(\frac{1}{\mathbf{p}_0} \odot \frac{\partial}{\partial\theta_i}\mathbf{p}_0 \odot \frac{\partial}{\partial\theta_j}\mathbf{p}_0\right)}_{\text{information in initial distribution}} + \underbrace{\mathbb{1}^{\mathrm{T}}\left(\sum_{k=0}^{N_t-1}\mathbf{Z}^{(\alpha\beta)}\mathbf{P}^k\right)\mathbf{p}_0}_{\text{information in state transitions}}. \tag{S24}$$

The matrix $\mathbf{Z}^{(\alpha\beta)}$ presents some mathematical issues, because it contains terms that have $p(x^{(i)}|x^{(j)})$ in the denominator, which in principle could be zero. First, in some settings, transitions from $x_i$ to $x_j$ have zero probability for some $i$'s and $j$'s. These transitions should not provide information as they are not possible. For rare transitions, i.e. $p(x^{(i)}|x^{(j)})$ is very small but not 0. When rare transitions are more sensitive to changes in parameters, the term $\frac{\mathbf{S}^{\alpha}_{ij}\mathbf{S}^{\beta}_{ij}}{\mathbf{P}_{ij}}$ is not problematic, which we observe to be the case for the examples presented here.

## S4. COMPARING TIME-SERIES AND SNAPSHOT DATA

In general, Fisher information of independent, identically distributed data are simply summed to obtain the total information for a given experiment,

$$\mathcal{I}_{\text{total}} = \sum_{i=1}^{N_{\text{data}}} \mathcal{I}. \tag{S25}$$

In the case of snapshot data (as in [7, 8]), the data points are from individual, independent cells each time point, and therefore the total information can be written as

$$\mathcal{I}(\theta)^{ss}_{\alpha\beta} = \sum_{k=1}^{N_t} N_c(t_k) \sum_{l=1}^{N} \frac{1}{p(x_k^{(l)})} \partial_\alpha p(x_k^{(l)}) \partial_\beta p(x_k^{(l)}), \tag{S26}$$

where $N_c(t)$ is the number of cells measured at time $t$. Because different cells *must* be measured at different time points by the nature of these experiments, the total number of measurements increases naturally with the number of time points. For the path-based information calculation, the independent data object is not a point measurement as in Eq. S26, but instead is the entire trajectory, and therefore the number of cells that are measured does not necessarily scale with time, that is if all $N_c$ measured cells are of the same length, the total information is simply

$$\mathcal{I}(\theta)^{ts}_{\alpha\beta} = N_c \, \mathcal{I}^{ts}_{\alpha\beta}(\Delta t). \tag{S27}$$

In practice, there are certain types of measurement modalities which lend themselves to measuring many cells independently, for example smFISH [9, 10]. In such experiments, cells are *fixed* or killed in the measurement process. Therefore, measurements are necessarily independent in time. This contrasts live-cell imaging experiments, such as individual RNA imaged using the MS2 platform [11], in which numbers of molecules are tracked over time in individual cells.

## S5. CONTINUOUS TIME BIRTH-DEATH PROCESS

Here we consider the classic immigration-death or birth-death system, which has been used to model constitutively expressed genes in numerous organisms [12, 13]. The system consists of two events, production and degradation of some molecule $X$, which occur with

rates $\theta = [k_r, \gamma]$

$$\varnothing \xrightarrow{k_r} X \tag{S28}$$

$$X \xrightarrow{\gamma} \varnothing \tag{S29}$$

The generator matrix is then truncated to only include the first $N$ molecules using the FSP approach in Eq. S3 as

$$\mathbf{A} = \begin{bmatrix} -k_r & \gamma & 0 & 0 & \ddots \\ k_r & -k_r - \gamma & 2\gamma & 0 & \ddots \\ 0 & k_r & -k_r - 2\gamma & 3\gamma & \ddots \\ \vdots & \ddots & \ddots & \ddots & \ddots \\ 0 & \dots & \dots & k_r & -k_r - N\gamma \end{bmatrix}. \tag{S30}$$

We used the formulation of transition probabilities described in Eq. S7 to compute the transition probability matrix for any given $t$ and $dt$, i.e. the matrix $\mathbf{P}$. From there, we can apply Eq. S24, and find the Fisher information. In lieu of an analytical form of the FIM, we use asymptotic normality of the maximimum likelihood estimator to check the FIM numerically. This relies on obtaining maximum likelihood estimates for many different realizations of data, and comparing the variance of the MLEs to the inverse of the FIM. First, we applied this to a single-parameter example as in the discrete time decay process above. For each of the 1,000 trajectories we find the value of $k_r$ which maximizes the likelihood in Eq. S10.

## S6. TWO-STATE GENE EXPRESSION MODEL

A two-state gene expression model has been used to describe rich biological phenomena [14, 15]. We consider a system with four reactions,

$$\begin{aligned} &\mathcal{G}_{\text{off}} \xrightarrow{k_{\text{on}}} \mathcal{G}_{\text{on}}; \quad \mathcal{G}_{\text{on}} \xrightarrow{k_{\text{off}}} \mathcal{G}_{\text{off}} \\ &\mathcal{G}_{\text{on}} \xrightarrow{k_{\text{r}}} \mathcal{G}_{\text{on}} + \text{RNA}; \quad \text{RNA} \xrightarrow{\gamma} \varnothing. \end{aligned} \tag{S31}$$

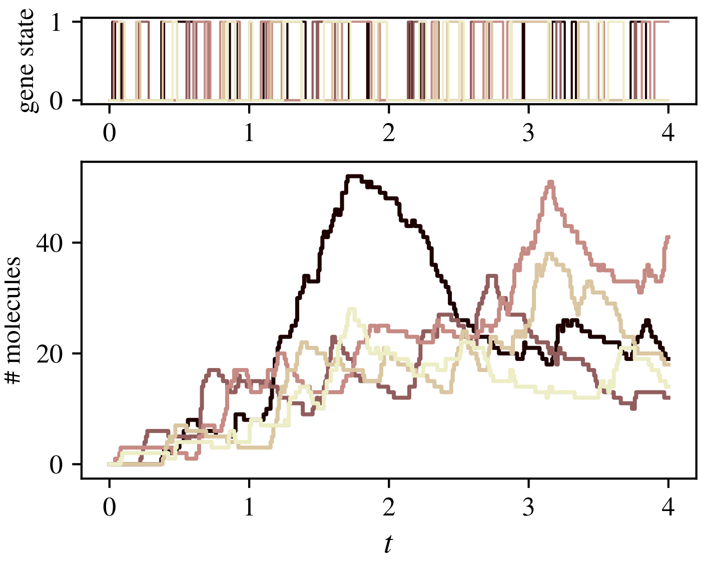


FIG. S1. Sample trajectories for the two-state gene expression model. The top panel shows the gene state for five trajectories and the bottom panel shows the corresponding mRNA trajectories.

From this description, we can construct a generator matrix for the finite number of molecules of mRNA $N$ as

$$\mathbf{G} = \begin{bmatrix} -k_{\text{on}} - k_{\text{off}} & k_{\text{on}} \\ k_{\text{off}} & -k_{\text{on}} - k_{\text{off}} \end{bmatrix}, \mathbf{K} = \begin{bmatrix} k_r & 0 \\ 0 & k_r \end{bmatrix}, \mathbf{\Gamma} = \begin{bmatrix} \gamma & 0 \\ 0 & \gamma \end{bmatrix} \tag{S32}$$

$$\mathbf{A} = \begin{bmatrix} \mathbf{G}-\mathbf{K} & \mathbf{\Gamma} & \mathbf{0} & \mathbf{0} & \ddots \\ \mathbf{K} & \mathbf{G}-\mathbf{K}-\mathbf{\Gamma} & 2\mathbf{\Gamma} & \mathbf{0} & \ddots \\ \mathbf{0} & \mathbf{K} & \mathbf{G}-\mathbf{K}-2\mathbf{\Gamma} & 3\mathbf{\Gamma} & \ddots \\ \vdots & \ddots & \ddots & \ddots & \ddots \\ \mathbf{0} & \dots & \dots & \mathbf{K} & \mathbf{G}-\mathbf{K}-N\mathbf{\Gamma} \end{bmatrix}. \tag{S33}$$

To further validate the trajectory based Fisher information, we began by using the stochastic simulation algorithm [16] to simulate 500 trajectories of the system with $\Delta t = 0.1$ and $N_t = 100$. Five example trajectories are shown in Fig. S1. The parameters were chosen as $k_{\text{on}} = 5$, $k_{\text{off}} = 15$, $k_r = 100$ relative to a characteristic decay rate $\gamma = 1$. We consider the Fisher information for fully observable states, in which both the gene state and the mRNA are observed, and validate the FIM using the asymptotic normality of the maximum likelihood estimator as we did with the birth-death system. First, we consider only one free parameter, $k_r$, as we did for the birth-death process in the previous example. The histogram

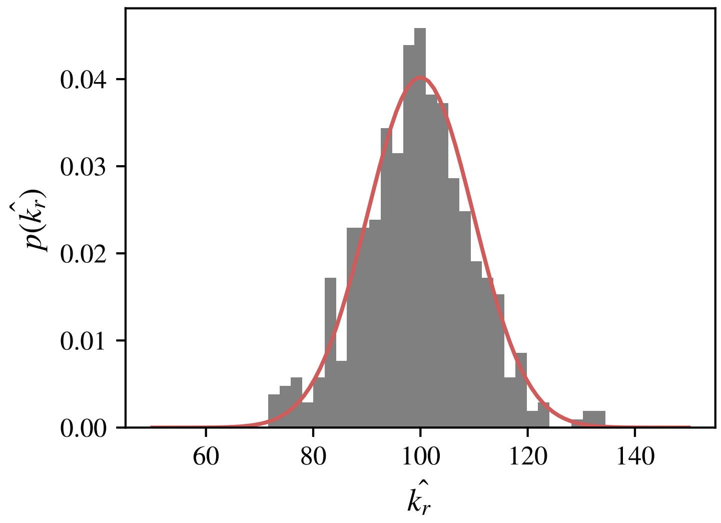


FIG. S2. *Verification of the Fisher information for the bursting gene model with a single parameter.* Distribution of maximum likelihood estimates (grey) and a Gaussian distribution (red) for the parameter $k_r$ with variance given by $\frac{1}{\mathcal{I}^{ts}}$ for $\hat{k}_r$. Trajectories were generated with parameters $k_r = 100$, $\gamma = 1$, $k_{\text{on}} = 5$, $k_{\text{off}} = 15$.

is shown in Fig. S2, where the black line denotes a Gaussian distribution with variance given by $\frac{1}{\mathcal{I}^{ts}}$. We also fit the same data with $\theta = [k_r, k_{\text{on}}, k_{\text{off}}]$, and show the maximum likelihood estimates for each trajectory as gray dots in Fig. S4. The 95% confidence intervals are calculated from the Cramér-Rao bound, i.e. $(\mathcal{I}^{ts})^{-1}$.

## S7. RELATING FISHER INFORMATION AND CHANNEL CAPACITY

Biological systems are constantly responding to their environments, and processing information about the environment or current cell state is critical to maintaining life [17]. Much work in the last decade has studied the information processing ability of various biomolecular systems, with particular emphasis on signal transduction pathways and transcription factor networks [17–24]. Typically, such studies aim to compute the mutual information between the input $X$ and output $Y$, defined as

$$I(X;Y) = H(X) - H(X|Y) \tag{S34}$$

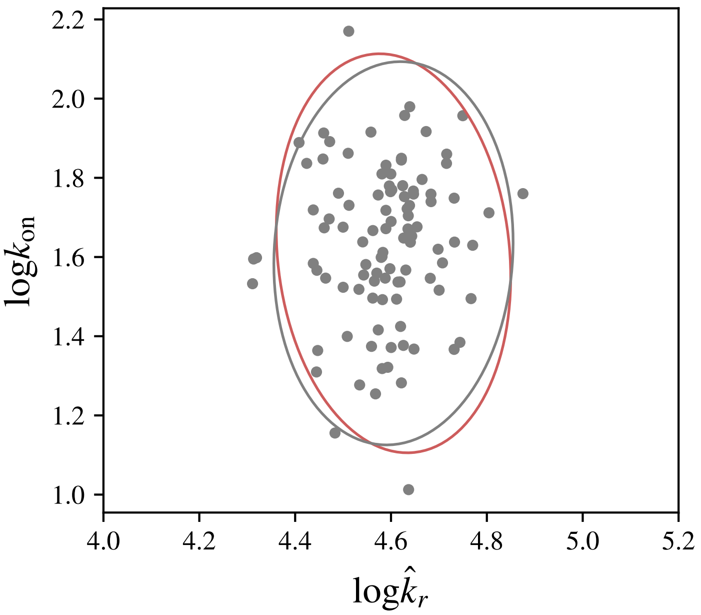


FIG. S3. *Verification of the Fisher information for the bursting gene model with two free parameters.* Distribution of maximum likelihood estimates (grey dots) for $k_r$ and $k_{\text{on}}$. The 95% CI for the estimated parameters was estimated from the MLE estimates as the grey ellipse and with the covariance given by $\mathcal{I}^{ts-1}$. Trajectories were generated with parameters $k_r = 100$, $\gamma = 1$, $k_{\text{on}} = 5$, $k_{\text{off}} = 15$.

where $H(\cdot) = \sum p(\cdot) \log_2 p(\cdot)$ is the entropy of the random variable. By determining the input distribution $P(X)$ which maximizes the mutual information, one can determine the channel capacity $\mathcal{C}$ of the system where $\mathcal{C}$ has units of bits. By Shannon's coding theorem [25], this means that the output $Y$ can accurately distinguish $2^{\mathcal{C}}$ distinct inputs.

In this section, we show how the Fisher information for CTMC's can be used to calculate channel capacities using a quantitative relationship between the mutual information and Fisher information. This approach has been discussed in the context of neuroscience [26], and more recently used for complex stochastic biochemical signaling [23]. As noted in [23], this approach generalizes well to multi-dimensional inputs, time-series outputs, and does not require assumptions about the nature of the output distribution. We refer the reader to [23, 26] for a full derivation relating the Fisher information to the mutual information, but outline the key results here.

Consider a collection of $N$ cells which receive a stimulus $X$ which is processed by, for

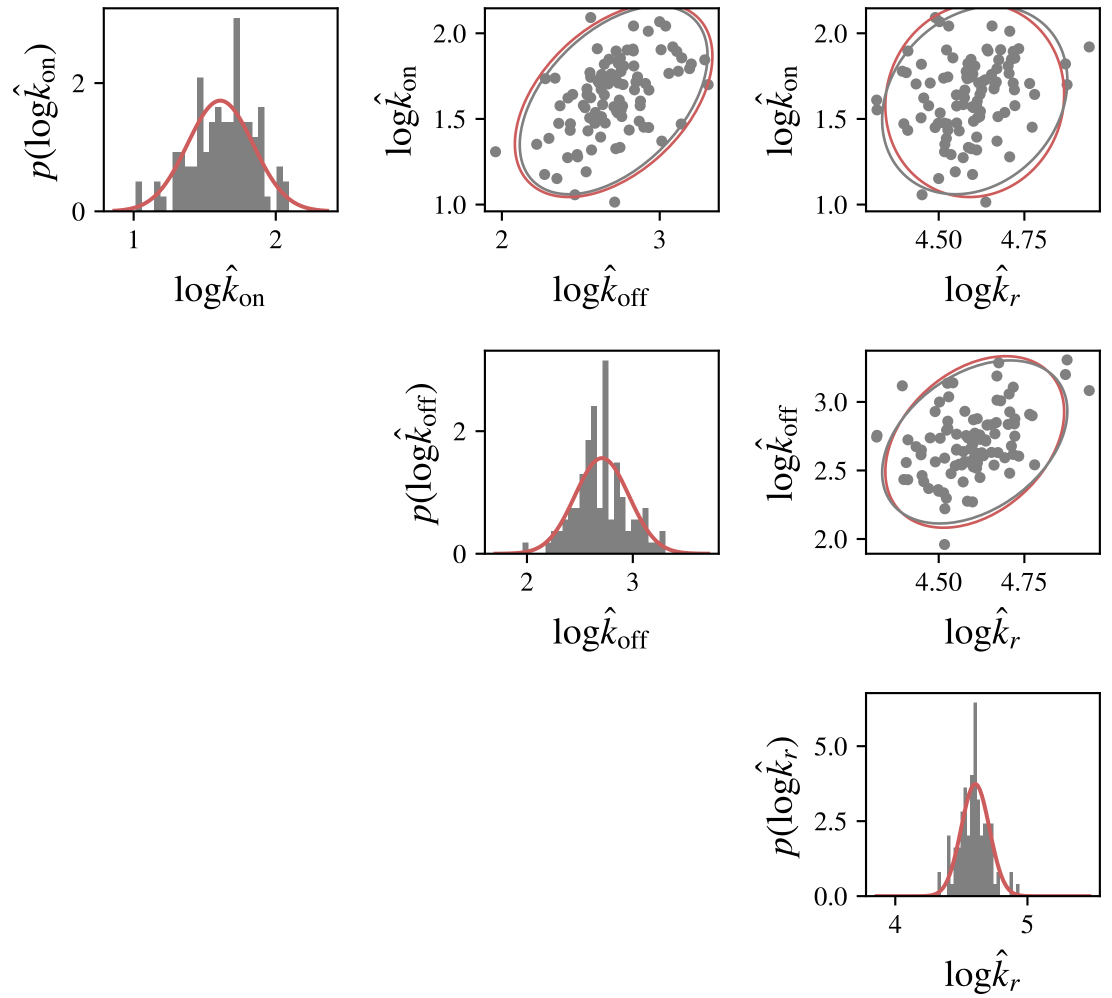


FIG. S4. *Verification of the Fisher information for the bursting gene model with three free parameters.* Distribution of maximum likelihood estimates (grey dots) for $k_r$, $k_{\text{off}}$ and $k_{\text{on}}$. The 95% CI for the estimated parameters was estimated from the MLE estimates as the grey ellipse and with the covariance given by ${\mathcal{I}^{ts}}^{-1}$. Trajectories were generated with parameters $k_r = 100$, $\gamma = 1$, $k_{\text{on}} = 5$, $k_{\text{off}} = 15$.

example a transcription factor network, and the output is a stochastic time-series $\vec{Y}$ for each cell, i.e. $\mathbf{Y} = [\vec{Y}_1, \vec{Y}_1, \ldots, \vec{Y}_N]$. Intuitively, the question of information processing by this collection of cells amounts to quantifying how precisely $X$ can be estimated from $\mathbf{Y}$. As discussed throughout the manuscript, the inverse of the Fisher information $\mathcal{I}^{-1}(X)$ gives the lower bound on any unbiased estimator of $X$, i.e. the Cramér-Rao bound [5]. Thus, the

mutual information between $X$ and $\hat{X}$ is given by

$$I(X;\mathbf{Y}) \geq I(X;\hat{X}) = H(\hat{X}) - \int dXp(X)H(\hat{X}|X), \tag{S35}$$

where the $I(X;\mathbf{Y}) \geq I(X;\hat{X})$ stems from the information processing inequality. When there are a sufficient number of cells, we have shown before that the maximum likelihood estimator has a normal distribution with a variance given by $\frac{1}{N\cdot\mathcal{I}(X)}$, and therefore we can write the entropy of the estimator as a Gaussian,

$$I(X;\mathbf{Y}) \approx H(\hat{X}) - \int dXp(X)\frac{1}{2}\log\frac{2\pi e}{N\cdot\mathcal{I}(\mathcal{X})}. \tag{S36}$$

Finally, if the estimator is efficient and has low variance, as is the case when $\mathcal{I}(X) >> 1$, then the entropy of the estimator is essentially governed by the entropy of the input, so $H(X) \approx H(\hat{X})$. Therefore, we have the expression for the approximate mutual information given by

$$I(X;\mathbf{Y}) \approx H(X) - \int dXp(X)\frac{1}{2}\log\frac{2\pi e}{N\cdot\mathcal{I}(X)}. \tag{S37}$$

Finally, using the theory of reference priors, it can be shown that the Jeffrey's prior is the one that maximizes mutual information between input and output [27]; that is

$$p(X) = \frac{1}{Z}\sqrt{\mathcal{I}(X)} \tag{S38}$$

where $Z = \int dX'\sqrt{\mathcal{I}(X')}$ Therefore, by plugging the above equation into Eq. S37, the approximate channel capacity can be found,

$$\mathcal{C}_{\text{total}} = \frac{1}{2}\log_2 N + \log_2\left(2\pi e^{-\frac{1}{2}}\int dX'\sqrt{\mathcal{I}(X')}\right). \tag{S39}$$

The first term describes how the channel capacity scales with number of cells, and the second term describes the contribution of each individual cell to the overall channel capacity [23]. In that sense, we call the individual contribution

$$\mathcal{C}_{\text{ind}} = \log_2\left(2\pi e^{-\frac{1}{2}}\int dX'\sqrt{\mathcal{I}(X')}\right). \tag{S40}$$

For a fixed population of cells, we can see that only $\mathcal{C}_{\text{ind}}$ is a function of $X$, and therefore we will see how this term is affected by different kinetic model parameters. Next, we apply this to a simple non-linearly regulated gene.

**A simple regulated gene**

To show how this may be used to determine the channel capacity of gene regulatory network, we begin with a simple regulated gene product $Y$, which undergoes two reactions:

$$\varnothing \xrightarrow{k_0 + k_{\max}\frac{x^n}{K_d^n + x^n}} Y$$
$$Y \xrightarrow{\gamma} \varnothing. \tag{S41}$$

The gene product $Y$ is regulated by some upstream signaling molecule or transcription factor $x$, as shown in Fig. S5, in a similar framework to [28]. We analyze the channel capacity of this system for different parameter values $\lambda = [k_0, n]$, shown in Fig. S5(b) by changing $k_0$ and $n$. For example, if $k_{\max} \gg k_0$ and $n \gg 0$ i.e. $\lambda_1$ in Fig. S5(b,e-f), the Hill activation function is approximately a step function, and thus we expect to differentiate between between two levels of $x$: those below $K_d$ and those above $K_d$. Consistent with this intuition, we found $\mathcal{C}_{\text{ind}} = 2.01$ for $\lambda_1$. When the response is linear, for example for the parameter set $\lambda_2 = [2.0, 1.5]$, the mitigating factor in discerning between inputs is the scale of the fluctuations of each trajectory, and find $\mathcal{C}_{\text{ind}}$ to be 4.4.

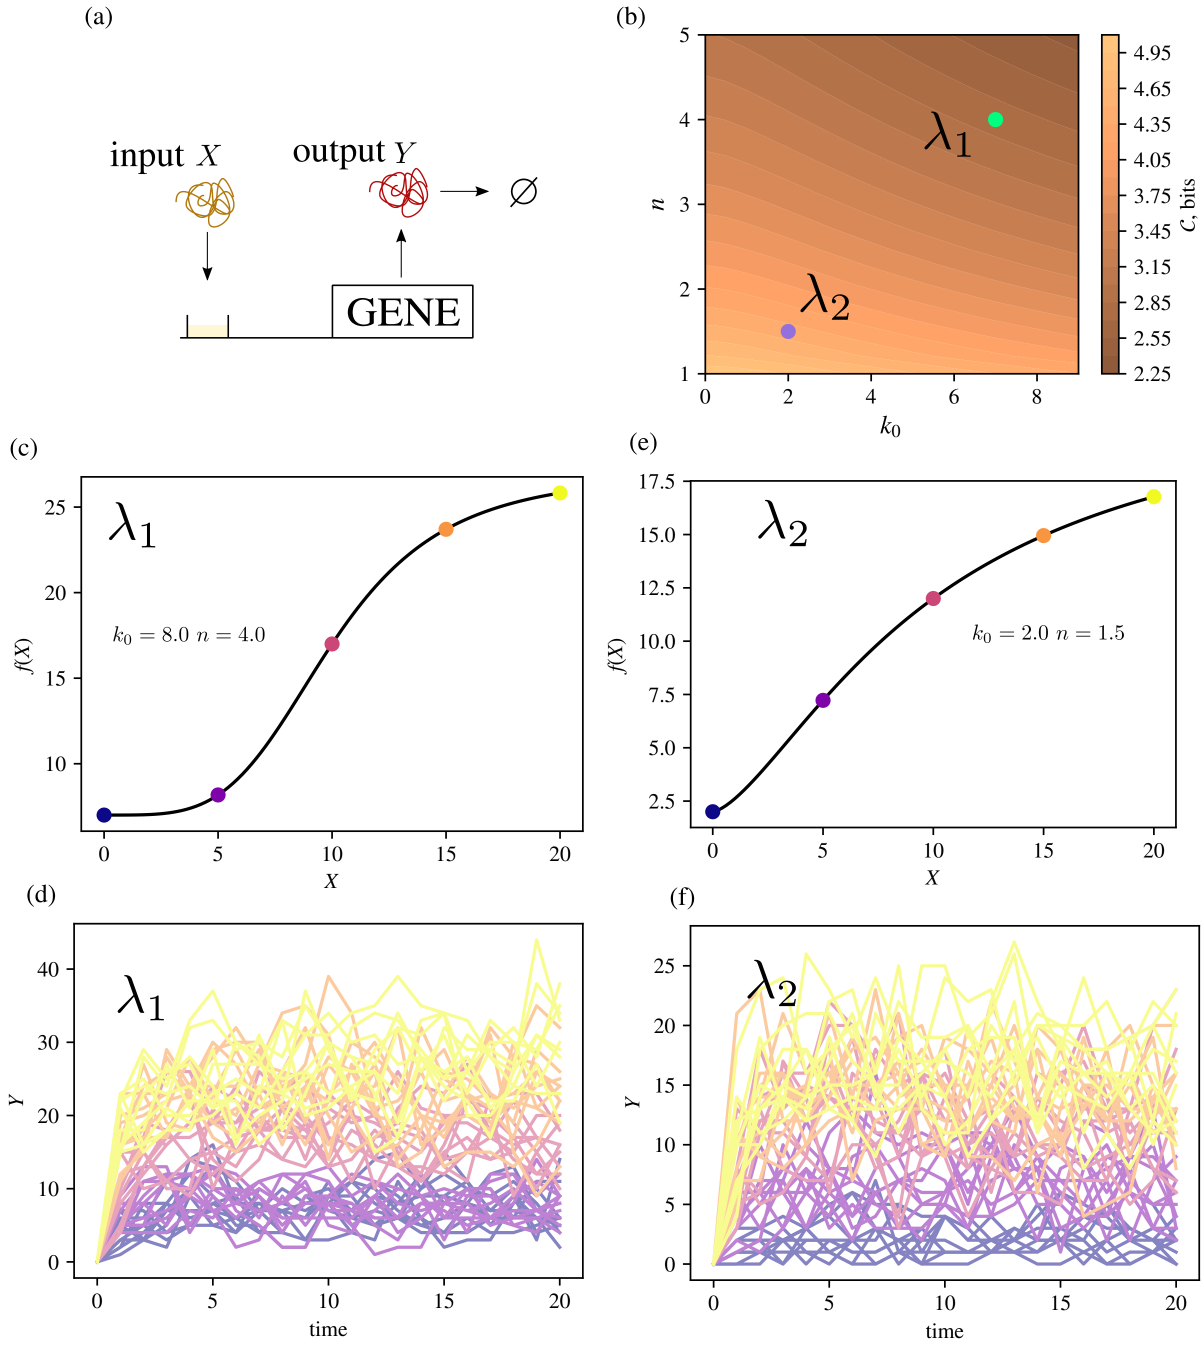


FIG. S5. Channel capacity calculations for a simple regulated gene. (a) schematic of the gene regulatory network. (b) Channel capacity as a function of model parameters $k_0$ and $n$. (c,e) Regulatory function curve, $f(X)$ as a function of $X$. Colored dots correspond to different values of $X$. (d,e) Five simulated trajectories for each of the parameters $\lambda_1$ and $\lambda_2$. Each trajectory is colored according to the value of the input $X$ in panels (c,e).

[1] W. J. Anderson, *Continuous-time Markov chains: An applications-oriented approach* (Springer Science & Business Media, 2012).

[2] N. G. Van Kampen and N. Godfried, *Stochastic processes in physics and chemistry* (Elsevier, 1992).

[3] D. A. McQuarrie, Stochastic Approach to Chemical Kinetics, Journal of Applied Probability **4**, 413 (1967).

[4] B. Munsky and M. Khammash, The finite state projection algorithm for the solution of the chemical master equation., The Journal of Chemical Physics **124**, 044104 (2006).

[5] S. M. Kay, *Fundamentals of Statistical Signal Processing: Estimation Theory* (Prentice-Hall, Inc., Upper Saddle River, NJ, USA, 1993).

[6] K. R. Haas, H. Yang, and J.-W. Chu, Fisher information metric for the langevin equation and least informative models of continuous stochastic dynamics, The Journal of Chemical Physics **139**, 121931 (2013).

[7] Z. R. Fox and B. Munsky, The finite state projection based Fisher information matrix approach to estimate information and optimize single-cell experiments., PLoS computational biology **15**, e1006365 (2019).

[8] Z. R. Fox, G. Neuert, and B. Munsky, Optimal Design of Single-Cell Experiments within Temporally Fluctuating Environments, Complexity **2020**, 1 (2020).

[9] A. M. Femino, F. S. Fay, K. Fogarty, and R. H. Singer, Visualization of single RNA transcripts in situ., Science **280**, 585 (1998).

[10] A. Raj, C. S. Peskin, D. Tranchina, D. Y. Vargas, and S. Tyagi, Stochastic mRNA synthesis in mammalian cells., PLoS biology **4**, e309 (2006).

[11] I. Golding, J. Paulsson, S. M. Zawilski, and E. C. Cox, Real-time kinetics of gene activity in individual bacteria., Cell **123**, 1025 (2005).

[12] Zenklusen, D, Larson, D R, and Singer, R H, Single-RNA counting reveals alternative modes of gene expression in yeast., Nature structural & molecular biology **15**, 1263 (2008).

[13] B. Munsky, G. Neuert, and A. van Oudenaarden, Using gene expression noise to understand gene regulation, Science **336**, 183 (2012).

[14] J. Peccoud and B. Ycart, Markovian modeling of gene-product synthesis, Theoretical Population Biology **48**, 222 (1995).

[15] V. Shahrezaei and P. S. Swain, Analytical distributions for stochastic gene expression, Proceedings of the National Academy of Sciences **105**, 17256 (2008).

[16] D. T. Gillespie, Exact stochastic simulation of coupled chemical reactions, The Journal of Physical Chemistry **81**, 2340 (1977).

[17] A. Levchenko and I. Nemenman, Cellular noise and information transmissionenglish, Current Opinion in Biotechnology **28**, 156 (2014).

[18] T. Gregor, D. W. Tank, E. F. Wieschaus, and W. Bialek, Probing the Limits to Positional Information, Cell **130**, 153 (2007).

[19] A. M. Walczak, G. Tkačik, and W. Bialek, Optimizing information flow in small genetic networks. II. Feed-forward interactions, Physical Review E **81**, 041905 (2010).

[20] R. Cheong, A. Rhee, C. J. Wang, I. Nemenman, and A. Levchenko, Information transduction capacity of noisy biochemical signaling networks., Science (New York, N.Y.) **334**, 354 (2011).

[21] T. Mora, Physical Limit to Concentration Sensing Amid Spurious Ligands, Physical Review Letters **115**, 038102 (2015).

[22] T. Mora and I. Nemenman, Physical Limit to Concentration Sensing in a Changing Environment, Physical Review Letters **123**, 198101 (2019).

[23] T. Jetka, K. Nienałtowski, S. Filippi, M. P. H. Stumpf, and M. Komorowski, An information-theoretic framework for deciphering pleiotropic and noisy biochemical signaling., Nature Communications **9**, 4591 (2018).

[24] M. Vennettilli, S. Saha, U. Roy, and A. Mugler, Precision of protein thermometry, Physical Review Letters **127**, 098102 (2021).

[25] C. E. Shannon, A mathematical theory of communication, The Bell System Technical Journal **27**, 379 (1948).

[26] N. Brunel and J.-P. Nadal, Mutual Information, Fisher Information, and Population Coding, Neural Computation **10**, 1731 (1998).

[27] J. J. Rissanen, Fisher information and stochastic complexity, IEEE transactions on information theory **42**, 40 (1996).

[28] G. Tkačik, A. M. Walczak, and W. Bialek, Optimizing information flow in small genetic networks, Physical Review E **80**, 031920 (2009).
